# Supplementary material for: First Measurement of Inclusive Electron-Neutrino and Antineutrino Charged Current Differential Cross Sections in Charged Lepton Energy on Argon in MicroBooNE
Source: arXiv:2109.06832 ancillary file (2022-02-03)
Supplement: Supplementary file 1 [file Supplemental_Material.pdf]

# Supplementary Material: First Measurement of Inclusive Electron-Neutrino and Antineutrino Charged Current Differential Cross Sections in Charged Lepton Energy on Argon in MicroBooNE

(Dated: February 3, 2022)

## Cross Section Values Energy

The values of the unfolded data cross section as a function of electron or positron energy are given in Table I. This table also includes the efficiency for  $\nu_e$  and  $\bar{\nu}_e$  in each bin. The generator predictions, provided in Table II, have been smeared by the corresponding additional smearing matrix,  $A_c$ .

TABLE I. The values of the unfolded data cross section as a function of electron or positron energy in each of the bins. The total uncertainty, obtained from the square-root of the diagonals for the unfolded covariance matrix, along with the efficiency for  $\nu_e$  and  $\bar{\nu}_e$  is given for each bin.

| Bin Num. | Energy Range | $d\sigma/dE_e$<br>( $10^{-39}$ cm <sup>2</sup> /GeV/nucleon) | Total Uncertainty<br>( $10^{-39}$ cm <sup>2</sup> /GeV/nucleon) | $\nu_e$ Efficiency | $\bar{\nu}_e$ Efficiency |
|----------|--------------|--------------------------------------------------------------|-----------------------------------------------------------------|--------------------|--------------------------|
| 1        | [0.00, 0.30) | 2.89                                                         | 1.30                                                            | 0.06               | 0.06                     |
| 2        | [0.30, 0.47) | 5.38                                                         | 1.82                                                            | 0.14               | 0.14                     |
| 3        | [0.47, 0.70) | 4.00                                                         | 1.05                                                            | 0.21               | 0.21                     |
| 4        | [0.70, 0.99) | 2.67                                                         | 0.66                                                            | 0.26               | 0.26                     |
| 5        | [0.99, 1.43) | 1.36                                                         | 0.40                                                            | 0.28               | 0.28                     |
| 6        | [1.43, 3.00) | 0.29                                                         | 0.09                                                            | 0.30               | 0.30                     |
| 7        | [3.00, 6.00) | 0.06                                                         | 0.04                                                            | 0.26               | 0.26                     |

TABLE II. The values of the generator cross section predictions as a function of electron or positron energy in each of the bins. These predictions have been smeared by the additional smearing matrix in electron or positron energy.

| Bin Num. | Energy Range | $d\sigma/dE_e$<br>GENIE v3.0.6 ( $\mu$ B Tune)<br>( $10^{-39}$ cm <sup>2</sup> /GeV/nucleon) | $d\sigma/dE_e$<br>GENIE v3.0.6<br>( $10^{-39}$ cm <sup>2</sup> /GeV/nucleon) | $d\sigma/dE_e$<br>NuWro v19.02.2<br>( $10^{-39}$ cm <sup>2</sup> /GeV/nucleon) | $d\sigma/dE_e$<br>GiBUU 2019<br>( $10^{-39}$ cm <sup>2</sup> /GeV/nucleon) |
|----------|--------------|----------------------------------------------------------------------------------------------|------------------------------------------------------------------------------|--------------------------------------------------------------------------------|----------------------------------------------------------------------------|
| 1        | [0.00, 0.30) | 2.74                                                                                         | 2.39                                                                         | 2.45                                                                           | 2.77                                                                       |
| 2        | [0.30, 0.47) | 5.36                                                                                         | 4.67                                                                         | 4.83                                                                           | 5.38                                                                       |
| 3        | [0.47, 0.70) | 4.23                                                                                         | 3.68                                                                         | 3.83                                                                           | 4.15                                                                       |
| 4        | [0.70, 0.99) | 3.05                                                                                         | 2.66                                                                         | 2.76                                                                           | 2.86                                                                       |
| 5        | [0.99, 1.43) | 1.66                                                                                         | 1.47                                                                         | 1.52                                                                           | 1.54                                                                       |
| 6        | [1.43, 3.00) | 0.34                                                                                         | 0.32                                                                         | 0.33                                                                           | 0.34                                                                       |
| 7        | [3.00, 6.00) | 0.08                                                                                         | 0.07                                                                         | 0.08                                                                           | 0.08                                                                       |

## Cross Section Values $\cos\beta$

The values of the unfolded data cross section as a function of electron or positron  $\cos\beta$  are given in Table III. This table also includes the efficiency for  $\nu_e$  and  $\bar{\nu}_e$  in each bin. The generator predictions, provided in Table IV, have been smeared by the corresponding additional smearing matrix,  $A_c$ .

TABLE III. The values of the unfolded data cross section as a function of electron or positron  $\cos\beta$  in each of the bins. The total uncertainty, obtained from the square-root of the diagonals for the unfolded covariance matrix, along with the efficiency for  $\nu_e$  and  $\bar{\nu}_e$  is given for each bin.

| Bin Num. | $\cos\beta$ Range | $d\sigma/d\cos\beta_e$<br>( $10^{-39}$ cm <sup>2</sup> /nucleon) | Total Uncertainty<br>( $10^{-39}$ cm <sup>2</sup> /nucleon) | $\nu_e$ Efficiency | $\bar{\nu}_e$ Efficiency |
|----------|-------------------|------------------------------------------------------------------|-------------------------------------------------------------|--------------------|--------------------------|
| 1        | [-1.00, 0.60)     | 0.83                                                             | 0.23                                                        | 0.12               | 0.10                     |
| 2        | [0.60, 0.79)      | 2.80                                                             | 1.28                                                        | 0.20               | 0.17                     |
| 3        | [0.79, 0.90)      | 8.46                                                             | 2.06                                                        | 0.20               | 0.19                     |
| 4        | [0.90, 0.95)      | 12.99                                                            | 3.84                                                        | 0.28               | 0.26                     |
| 5        | [0.95, 1.00)      | 17.55                                                            | 4.16                                                        | 0.33               | 0.31                     |

TABLE IV. The values of the generator cross section predictions as a function of electron or positron  $\cos\beta$  in each of the bins. These predictions have been smeared by the additional smearing matrix in electron or positron  $\cos\beta$ .

| Bin Num. | $\cos\beta$ Range | $d\sigma/d\cos\beta_e$<br>GENIE v3.0.6 ( $\mu$ B Tune)<br>( $10^{-39}$ cm <sup>2</sup> /nucleon) | $d\sigma/d\cos\beta_e$<br>GENIE v3.0.6<br>( $10^{-39}$ cm <sup>2</sup> /nucleon) | $d\sigma/d\cos\beta_e$<br>NuWro v19.02.2<br>( $10^{-39}$ cm <sup>2</sup> /nucleon) | $d\sigma/d\cos\beta_e$<br>GiBUU 2019<br>( $10^{-39}$ cm <sup>2</sup> /nucleon) |
|----------|-------------------|--------------------------------------------------------------------------------------------------|----------------------------------------------------------------------------------|------------------------------------------------------------------------------------|--------------------------------------------------------------------------------|
| 1        | [-1.00, 0.60)     | 0.89                                                                                             | 0.79                                                                             | 0.83                                                                               | 0.89                                                                           |
| 2        | [0.60, 0.79)      | 4.64                                                                                             | 4.11                                                                             | 4.31                                                                               | 4.65                                                                           |
| 3        | [0.79, 0.90)      | 7.69                                                                                             | 6.89                                                                             | 7.03                                                                               | 6.86                                                                           |
| 4        | [0.90, 0.95)      | 14.85                                                                                            | 13.26                                                                            | 13.62                                                                              | 13.50                                                                          |
| 5        | [0.95, 1.00)      | 20.36                                                                                            | 18.08                                                                            | 18.87                                                                              | 19.66                                                                          |

### Unfolded Covariance Matrix

The unfolded total data covariance matrix for the differential cross section as a function of the electron or positron energy and  $\cos\beta$  is shown in Fig. 1. These matrices include the statistical and systematic uncertainties. The values for the unfolded covariance matrices are provided in the attached text file: `MicroBooNE_NuMI_NueInclusive_UnfoldedCovariance.txt`.

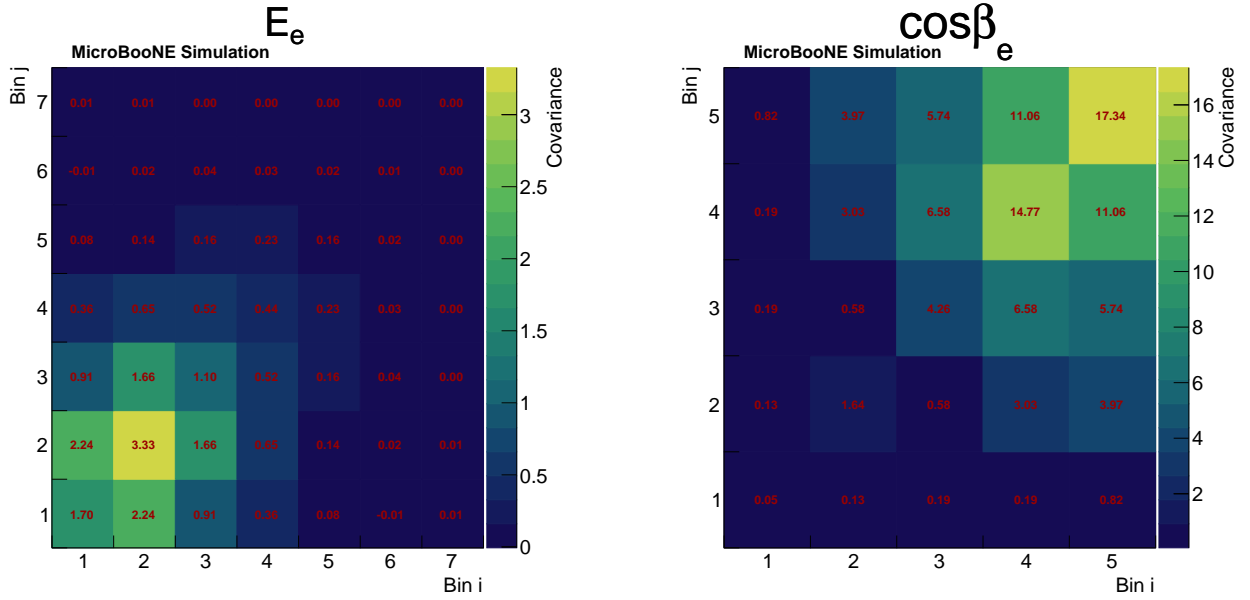

FIG. 1. The total unfolded data covariance matrix for (left) electron or positron energy and (right) electron or positron  $\cos\beta$ .

### Additional Smearing Matrix

Fig. 2 shows the additional smearing matrix  $A_c$  from the Wiener-SVD unfolding for electron or positron energy and  $\cos\beta$ . These matrices should be applied to the true differential cross section prediction when compared to the unfolded data differential cross section. The values for the additional smearing matrices are provided in the attached text file: MicroBooNE.NuMI.NueInclusive.Ac.txt.

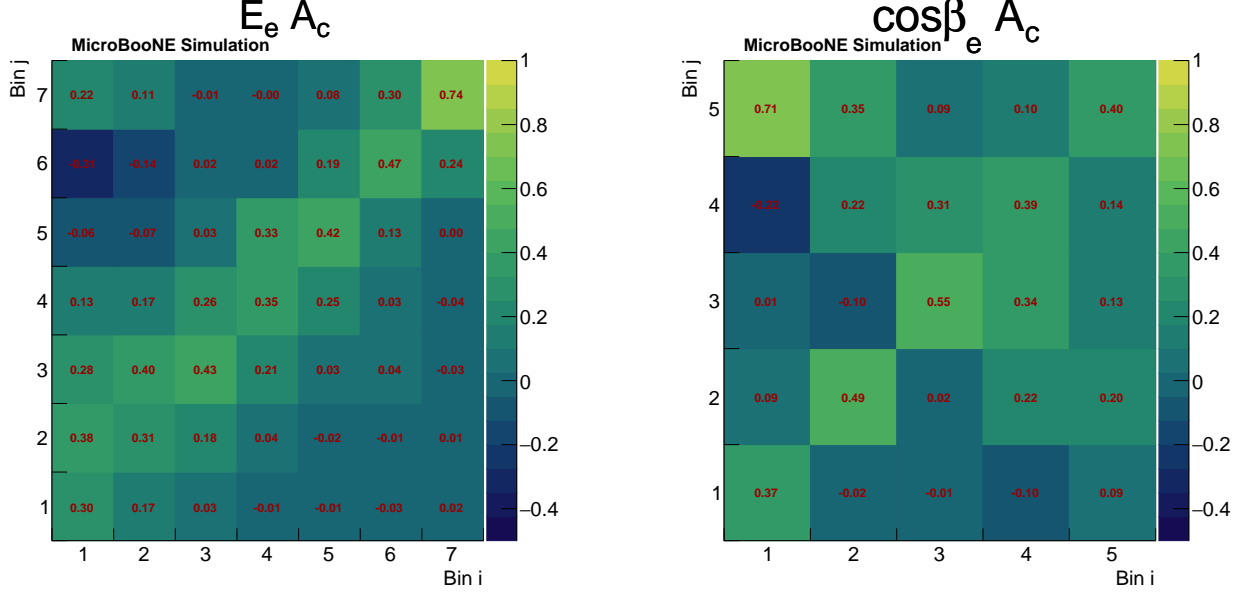

FIG. 2. The additional smearing matrix  $A_c$  returned by the Wiener-SVD unfolding for (left) electron or positron energy and (right) electron or positron  $\cos\beta$ .

### Efficiency

The efficiency broken down by neutrino interaction channel for electrons or positrons as a function of energy and  $\cos\beta$  is shown in Fig. 3. The measurement is sensitive to the charged-current (CC) quasi-elastic (QE), CC meson exchange current (MEC), CC resonant, and CC deep inelastic scattering neutrino interaction channels with a higher efficiency for selecting CC QE and CC MEC interactions.

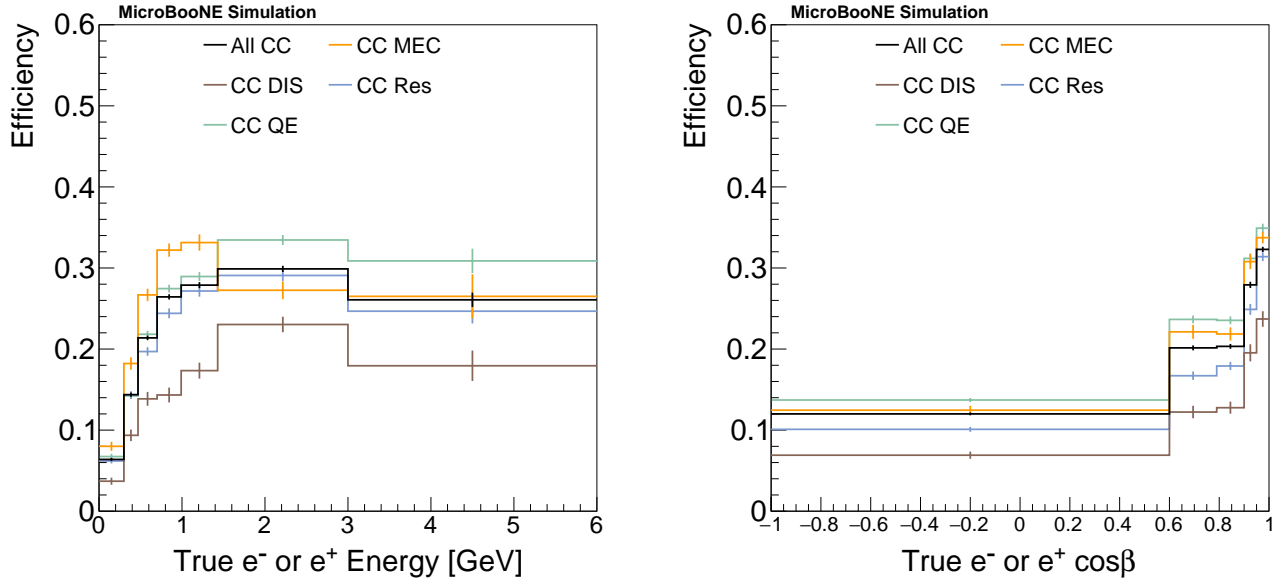

FIG. 3. The interaction mode efficiencies as a function of the (left) electron or positron energy and (right) electron or positron  $\cos\beta$ .

### Purity

The purity as a function of reconstructed electron or positron energy and  $\cos\beta$  is shown in Fig. 4. The purity is around 80% for most bins but with a lower purity for the lowest and highest energy bins.

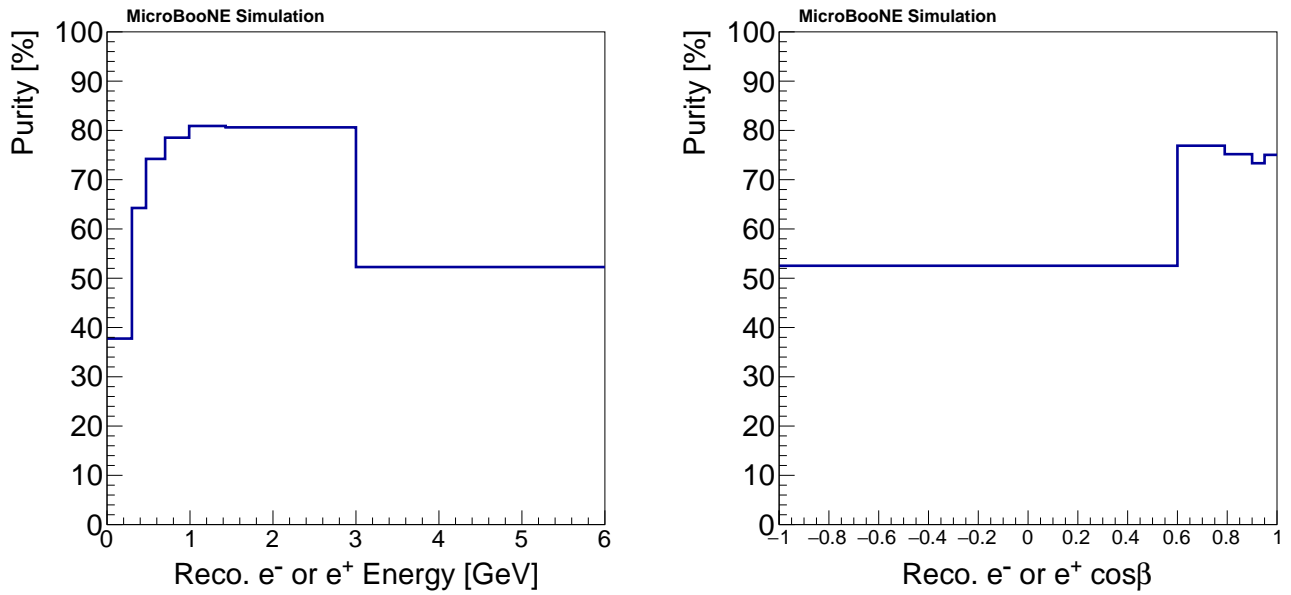

FIG. 4. The purity as a function of the electron or positron (left) energy and (right)  $\cos\beta$ .

## Uncertainties

The uncertainties in each bin broken down by type (before unfolding) as a function of reconstructed electron or positron energy and  $\cos\beta$  are shown in Fig. 5.

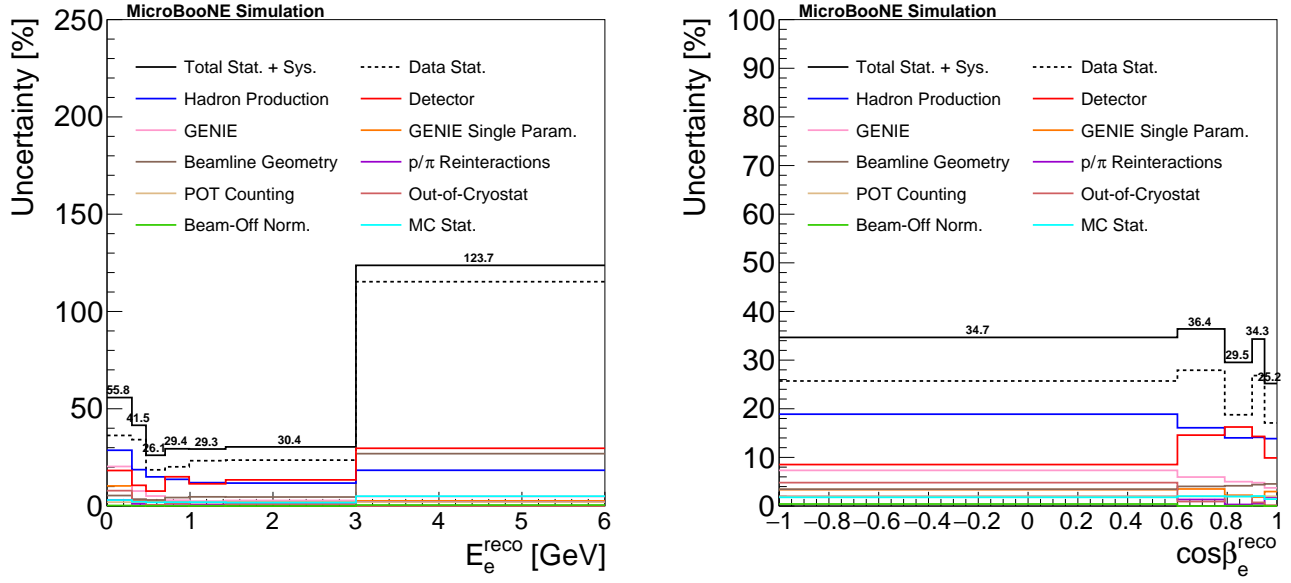

FIG. 5. The uncertainties broken down by type (before unfolding) as a function of the electron or positron (left) energy and (right)  $\cos\beta$ .

## Electron Neutrino and Antineutrino Flux

The individual  $\nu_e$  and  $\bar{\nu}_e$  fluxes as a function of neutrino energy are shown in Fig. 6. The values can be found in the `MicroBooNE_NuMI_NueFlux.txt` and `MicroBooNE_NuMI_NuebarFlux.txt` files. Figure 7 shows the ratio of the  $\nu_e$  and  $\bar{\nu}_e$  fluxes.

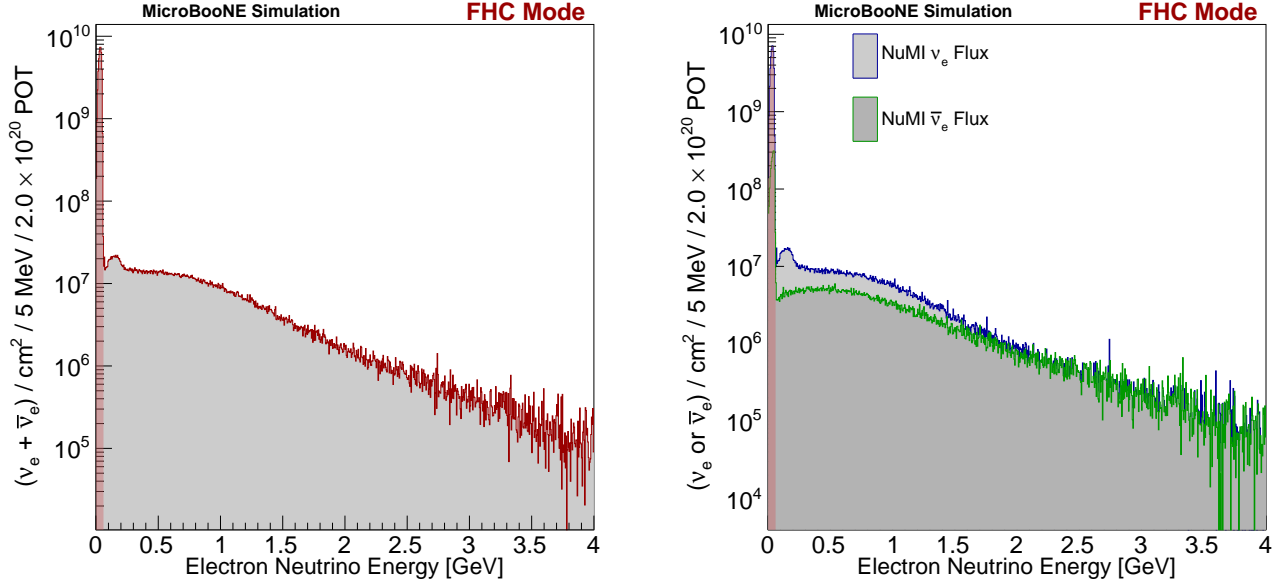

FIG. 6. The summed (left) and individual (right)  $\nu_e + \bar{\nu}_e$  NuMI flux at MicroBooNE as a function of the simulated neutrino energy. The masked out region in red shows the neutrino flux that is excluded by the 60 MeV neutrino energy threshold included in this measurement.

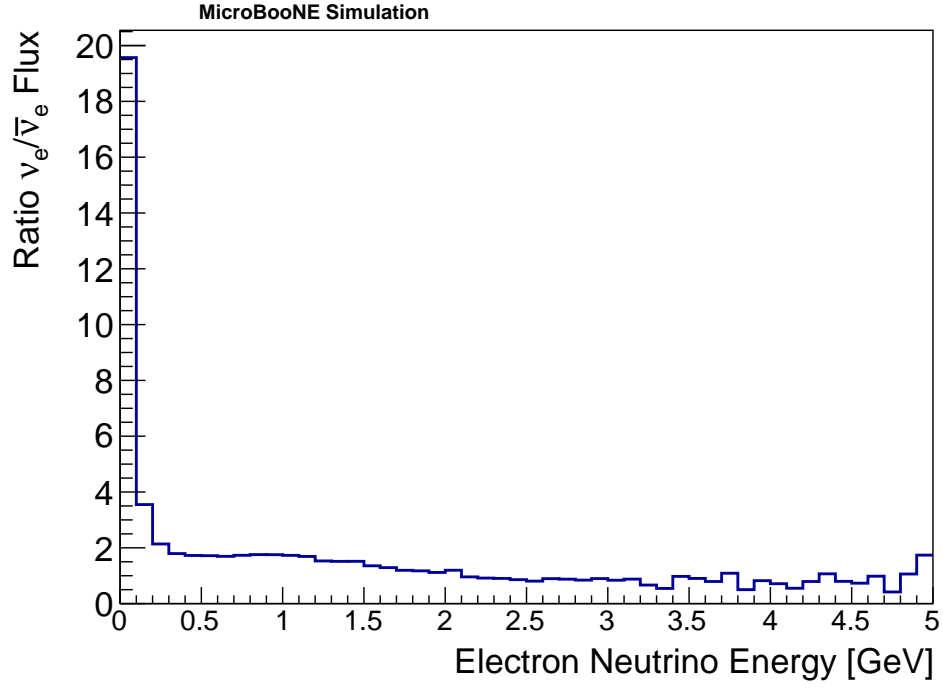

FIG. 7. The ratio of the  $\nu_e$  and  $\bar{\nu}_e$  NuMI neutrino fluxes at MicroBooNE as a function of simulated neutrino energy in 100 MeV bins. The large peak in the first bin is due to the significant  $\nu_e$  flux arising from muon decay-at-rest.
